# Supplementary material for: An extremely metal-deficient globular cluster in the Andromeda Galaxy
Source: arXiv:2010.07395 ancillary file (2020-10-14)
Supplement: Supplementary file 1 [file supplement.pdf]

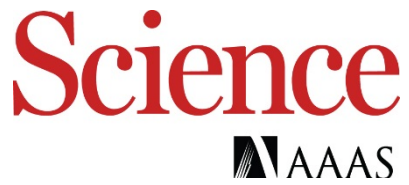

## Supplementary Materials for

An extremely metal-deficient globular cluster in the Andromeda Galaxy

Søren S. Larsen, Aaron J. Romanowsky, Jean P. Brodie, Asher Wasserman

Correspondence to: [s.larsen@astro.ru.nl](mailto:s.larsen@astro.ru.nl)

**This PDF file includes:**

Materials and Methods

Supplementary Text

Figures S1 to S3

Tables S1 to S10

## Materials and Methods

### Reduction of the spectra

The raw HIRES data were processed with the MAKEE (MAuna Kea Echelle Extraction) package (39). MAKEE takes as input the raw science frames, along with arc lamp spectra for wavelength calibration, bias frames, flat-fields, and a spectrum of a bright star for tracing of the echelle orders. It produces as output the final extracted one-dimensional spectra for each echelle order, with the wavelength scale corrected to the heliocentric reference frame. Once extracted by MAKEE, the two 1200 s exposures of EXT8 were averaged to an equivalent 2400 s exposure that was used in the further analysis.

To estimate the statistical uncertainties in the average spectrum, the two spectra were subtracted from each other; the uncertainty  $\sigma_{\langle P \rangle}$  on each mean pixel value  $\langle P \rangle$  was then estimated as  $\sigma_{\langle P \rangle} = |P_1 - P_2|/2$  where  $P_1$  and  $P_2$  are the pixel values in the individual spectra. Because the spectra used for the analysis were mapped to a linear wavelength scale by interpolation in the spectra extracted by the MAKEE software, the uncertainties of neighboring pixels become correlated, so that the difference spectrum underestimates the true uncertainties. The uncertainties estimated from the interpolated spectra were therefore multiplied by  $\sqrt{2}$  to account for this.

### Modeling of the integrated-light spectrum

We followed a published procedure for modeling of integrated-light spectra (16,18). Here we provide a brief summary with emphasis on aspects relevant to the analysis presented in this paper.

Clusters are modeled as simple stellar populations, i.e., as stellar populations characterized by a single age and composition. The Hertzsprung-Russell diagram (HRD), which describes the distribution of effective temperatures ( $T_{eff}$ ) and luminosities ( $L$ ) for the stars in the population, is first divided into a large number of bins (typically 50-100) covering the range of stellar properties that contribute to the cluster light. A model spectrum is then computed for each bin, and the model spectra are co-added with appropriate weights according to the number of stars in each bin. At each wavelength sampling point, the integrated-light monochromatic luminosity  $L_{SSP}(\lambda)$  is

$$L_{SSP}(\lambda) = \sum_{i=1}^n w_i L_i(\lambda), \quad (S1)$$

where the sum is over  $n$  bins of the HRD,  $w_i$  is the weight of the  $i$ th bin and  $L_i(\lambda)$  is the monochromatic luminosity at wavelength  $\lambda$  for a star in this bin. The weights are defined as

$$w_i = \xi(m_i) \Delta m_i, \quad (S2)$$

where  $\Delta m_i$  is the range of initial stellar masses covered by the  $i$ th bin and  $\xi(m) \equiv dN/dm$  is the stellar mass function for number of stars  $N$  and initial stellar mass  $m$ . We assume that  $\xi(m)$  follows a power-law of the form (40)

$$\xi(m) \propto \left( \frac{m}{0.5 M_{\odot}} \right)^{\alpha} \quad (\text{S3})$$

with  $\alpha = -2.3$  for  $m > 0.5 M_{\odot}$  and  $\alpha = -1.3$  for  $m < 0.5 M_{\odot}$ .

To find  $L_i(\lambda)$  for each bin, a model atmosphere is computed with the LINUX version of the ATLAS9 code (41-43), and a model spectrum is then computed with the SYNTHÉ spectral synthesis code (42-44). Because SYNTHÉ computes surface fluxes, the luminosities are obtained by scaling the fluxes according to the surface areas of the stars. The integrated-light model spectrum is scaled to match the same continuum level as the observed spectrum, and the abundances used in the modeling are adjusted until the best fit (minimum  $\chi^2$ ) is obtained. The modeling procedure is implemented as a PYTHON code, ISPY3 (37).

### Selection of isochrones for the modeling

The HRD bins used to model the spectrum of M15 (16) were defined based on photometry of individual stars obtained with the Hubble Space Telescope (HST). Because such data are not available for EXT8 and there are no Milky Way GCs with a similarly low metallicity, we used theoretical isochrones for our modeling of EXT8. Past analyses of extragalactic GCs have used isochrones from the Dartmouth group (45), which are available for the alpha-enhanced composition typical of old stellar populations. However, these isochrones are not available for metallicities  $[\text{Fe}/\text{H}] < -2.5$ . Therefore, we here used isochrones from the MIST group (20,46), which are available for metallicities as low as  $[\text{Fe}/\text{H}] = -4$ . The MIST isochrones, however, are only available for scaled-solar composition. At a fixed  $[\text{Fe}/\text{H}]$ , an increase in  $[\alpha/\text{Fe}]$  has an effect on the HRD that is very similar to that of an increase in the overall metal fraction (47,48), i.e., the isochrone shifts towards lower effective temperatures. An increase of about a factor of two in the abundances of the alpha-elements is equivalent to an increase of about 0.2 dex in the iron abundance  $[\text{Fe}/\text{H}]$  if the abundance ratios are kept scaled-solar (47). Hence, for our modeling of the spectra we used MIST isochrones for which  $[\text{Fe}/\text{H}]$  had been increased by about 0.2 dex relative to the iron abundance derived from the spectral analysis.

For  $[\text{Fe}/\text{H}] < -2$  and an age  $t$  of  $\log(t/\text{years})=10.10$  ( $t=12.5 \times 10^9$  years), a full MIST isochrone includes data for 556 points, covering all evolutionary phases from a lower mass limit of  $0.1 M_{\odot}$  on the main sequence to the tip of the asymptotic giant branch. From these, we selected 61 points along the isochrone for our modeling, which are listed in Table S1 for  $[\text{Fe}/\text{H}] = -2.7$ . The stellar masses, the effective temperatures, and the surface gravities ( $g$ ) were taken directly from the isochrone, while the stellar radii  $R$  followed from the bolometric luminosities  $L_{bol}$  and effective temperatures,

$$R/R_{\odot} = \left( \frac{L_{bol}}{L_{bol,\odot}} \right)^{1/2} \left( \frac{T_{eff,\odot}}{T_{eff}} \right)^2 \quad (\text{S4})$$

where  $R_{\odot}$ ,  $L_{bol,\odot}$ , and  $T_{eff,\odot}$  are the radius, bolometric luminosity, and effective temperature of the Sun. The bolometric luminosities are listed in solar units in the isochrones, while we assumed an effective temperature of 5777 K for the Sun (49). The weights were calculated as described above (equation S2), and Table S1 also lists, for each bin, the contribution to the continuum luminosity at 500 nm ( $L_{500\text{nm}}$ ). No single bin dominates the luminosity. Table S1 also lists the

values adopted for the microturbulent velocities in each bin, which depend on the surface gravity as described in (18).

### Measuring elemental abundances

The iron abundances were measured by fitting the 23 echelle orders in the wavelength range from 4400 Å – 6200 Å separately. Two orders, for which the model fitting did not converge, were rejected. The iron abundance was then obtained as an average of the values obtained from the model fitting to the remaining 21 orders, weighted by the inverse variance on each value, and the standard error on the mean was obtained from the dispersion of the measured values (18). With the iron abundance thus established, we then proceeded to model Ti, Ca, Mg, Si, Na, and K. Custom defined spectral ranges containing features from these elements were defined (Tables S4-S9) and model fitting was carried out separately for each spectral range.

An iron abundance of  $[\text{Fe}/\text{H}] = -2.39 \pm 0.02$  was previously measured for M15 when using HRD bins defined from the HST photometry (16). If we used the same M15 HRD bins as input for the modeling of EXT8, we found a mean iron abundance of  $[\text{Fe}/\text{H}] = -2.95 \pm 0.03$  (rms dispersion 0.153, 21 echelle orders), but this estimate is likely biased because EXT8 is more metal-poor than M15. To verify that the MIST isochrones give similar results as the analysis based on the empirical M15 CMD, we first used a MIST isochrone with  $[\text{Fe}/\text{H}] = -2.2$  and an age of  $12.5 \times 10^9$  years to model the spectra of both clusters. When including stars to the same magnitude limit as the empirical M15 HRD ( $M_V = +9$ ) we got the same iron abundance for M15 as before,  $[\text{Fe}/\text{H}] = -2.39$ , and for EXT8 we got  $[\text{Fe}/\text{H}] = -2.96$ . If we extended the isochrone to a faint limit of  $M_V = +12$ , the metallicities decreased slightly to  $[\text{Fe}/\text{H}] = -2.41$  for M15, and to  $[\text{Fe}/\text{H}] = -3.00$  for EXT8.

For our final model of the spectrum of EXT8, we used a MIST isochrone with a metallicity of  $[\text{Fe}/\text{H}] = -2.7$  and an age of  $12.5 \times 10^9$  years, with a faint limit of  $M_V = +12$ . This isochrone is then adequate for the iron abundance of  $[\text{Fe}/\text{H}] = -2.91$  and the alpha-enhancement of about a factor of two measured from the spectrum. The average abundances for each element are given in Table S2, and the individual measurements per echelle order (for  $[\text{Fe}/\text{H}]$ ) or spectral range (for the other abundances) are given in Tables S3-S9. The Na *D* lines are a special case, as they appear in two overlapping echelle orders in the HIRES spectrum. The  $[\text{Na}/\text{Fe}]$  value in Table S2 is the weighted average of the values obtained from the two model fits, but we list the two measurements separately in Table S4.

The opacity tables used to generate the ATLAS9 atmosphere models used in our analysis were calculated for a standard alpha-enhanced composition, which might lead to an inconsistency due to the large amount of Mg-depletion in EXT8. We have repeated the analysis using ATLAS12 models (43,50) in which the abundance patterns were taken into account self-consistently. For all elements, the abundances changed by less than 0.01 dex.

### Modeling the fraction of magnesium-poor stars

Our measurements of average abundances from the integrated-light spectrum of EXT8 do not directly constrain the underlying distribution of abundances that could produce these average values. To gain some insight into this, we modeled the strengths of the Mg *b* lines for composite populations with different  $[\text{Mg}/\text{Fe}]$  values. The equivalent width (EW) for a feature in an integrated-light spectrum is the luminosity-weighted average of the EWs in the individual stellar

spectra that make up the population (51, 52). We therefore used the Kurucz WIDTH9 code (43,50,53) to compute the EW for the Mg *b* lines for each of the HRD bins for different values of [Mg/Fe]. For the line at 5173 Å, we found integrated-light EWs of 55 mÅ, 98 mÅ and 151 mÅ for [Mg/Fe] = −1, −0.3 and +0.3, respectively. The EW of the population with [Mg/Fe] = −0.3 is close to a straight average of the EWs for populations with [Mg/Fe] = −1 and [Mg/Fe] = +0.3, implying that a roughly equal mix of populations with these abundances could produce the [Mg/Fe] value measured from the integrated light of EXT8. A very similar conclusion follows from analysis of the other two lines in the Mg *b* triplet. Other combinations are possible too. As one extreme, one could consider the limit in which the Mg abundance of the most Mg-poor population approaches zero, so that the Mg lines vanish. In this case, a mix of about 2/3 Mg-normal stars and 1/3 Mg-free stars would also reproduce the observations. It is also possible that the cluster only hosts a single population with the [Mg/Fe] value measured from the integrated-light spectrum, or the distribution of [Mg/Fe] values might be more complex.

### Radial velocity and velocity broadening

Prior to spectral fitting, the radial velocity was determined for each order by shifting the observed spectrum until the best fit to the model spectrum was obtained. In this way, an average velocity shift of  $-203.6 \text{ km s}^{-1}$  with an order-to-order dispersion of  $3.4 \text{ km s}^{-1}$  for 18 orders was obtained. This then gives a mean heliocentric radial velocity of  $-203.6 \pm 0.8 \text{ km s}^{-1}$  for EXT8.

The synthetic spectra were initially computed at a very high resolving power to fully sample the profiles of individual lines,  $R = 500\,000$ . The model spectra were then broadened to account for the instrumental resolution and the velocity dispersion of the stars in the cluster. This broadening was determined from an initial model fitting in which all abundance ratios were kept fixed at alpha-enhanced values, and the broadening required to match the observations was allowed to vary as a free parameter. We assumed that the broadening can be modeled as a convolution of the spectrum with a Gaussian kernel whose dispersion  $\sigma_\lambda$  is proportional to the wavelength. From 19 orders, we obtained an average broadening of  $\sigma_\lambda/\lambda = 4.58 \times 10^{-5}$  with a dispersion of  $1.19 \times 10^{-5}$ . Expressed as a velocity, this corresponds to an average broadening of  $13.7 \pm 0.8 \text{ km s}^{-1}$ . With the 1.15 arcsec slit, the instrumental broadening of the HIRES observations is  $R=37\,000$  according to the HIRES documentation (54), which is equivalent to a velocity dispersion of  $3.4 \text{ km s}^{-1}$ . When converting the resolving power  $R$  to a velocity dispersion, we have assumed that  $R$  represents the full width at half maximum (FWHM) of a Gaussian instrumental profile. Subtracting the instrumental dispersion in quadrature we then get a line-of-sight velocity broadening for EXT8 of  $\sigma = 13.3 \pm 0.8 \text{ km s}^{-1}$ .

### Cluster size and dynamical mass

Using the virial theorem, the velocity dispersion can be used to estimate the cluster mass. This also requires an estimate of the cluster size, which we obtained from archival images of EXT8 obtained with MegaCam on the Canada-France-Hawaii Telescope. We downloaded three images obtained on Nov 6, 2016 (P.I. M. Arnaboldi) in the Sloan Digital Sky Survey *g* filter, each with an exposure time of 100 s. EXT8 was identifiable as an extended object in these images, which had a FWHM seeing of 4.7-4.9 pixels or about 0.9 arcsec. To measure the intrinsic size of the cluster, we used the ISHAPE task in the BAOLAB package (38) to fit King profiles (55) convolved with the point-spread function (PSF).

Figure S1 shows the MegaCam image, the best-fitting King model convolved with the PSF, and the residuals. There is some substructure visible in the residual image, due to individual stars (in the outer regions) and imperfect modeling of the profile (near the center). The results are listed in Table S10 for each of the three MegaCam images and for three fitting radii (25 pixels = 4.6 arcsec, 50 pixels = 9.25 arcsec, and 100 pixels = 18.5 arcsec). The tidal radii are sensitive to the fitting radius, and only the largest fitting radius fully includes the cluster profile out to the measured tidal radius. However, the PSF is poorly constrained at radii greater than 25 pixels, so that the modeling of the cluster profile must be considered increasingly uncertain beyond this radius. The analytical King models used by ISHAPE may not exactly reflect the true profile. Hence, increasing the fitting radius does not necessarily lead to a more accurate estimate of the half-light radius.

The half-light radii are listed in Table S10, where  $R_{eff}(\text{ell})$  is the semi-major axis of an ellipse containing half of the cluster light, and  $R_{eff}(\text{circ})$  is the radius of a circular aperture that contains half of the light of the actual elliptical profile. For an assumed distance of 783 kpc (56), these correspond to physical half-light radii between  $R_{eff}(\text{circ}) = 2.52$  pc (for a fitting radius of 25 pixels) and  $R_{eff}(\text{circ}) = 2.98$  pc (for 100 pixels). We use the intermediate value measured in the 50 pixels aperture ( $R_{eff}(\text{circ}) = 2.77$  pc) and adopt 0.2 pc as an estimate of the uncertainty. The dynamical mass can now be calculated as

$$M_{dyn} = \eta \frac{R_{eff} \sigma^2}{G} \quad (\text{S5})$$

where the constant  $\eta \approx 10$  (57). Inserting our measurements of the velocity dispersion and radius, we obtain  $M_{dyn} = (1.14 \pm 0.16) \times 10^6 M_{\odot}$ , where the uncertainty on the derived mass is dominated by the uncertainty on the velocity dispersion.

#### Conversion from [Z/H] to [Fe/H]

The proposed metallicity floor for GCs is usually quoted in terms of the iron abundance, [Fe/H], while the E-MOSAICS simulation (36) quantifies metallicity in terms of the total abundance of elements heavier than He, [Z/H]. To convert between the two, we added 0.2 dex to the proposed metallicity floor at [Fe/H] = -2.5 (47), so that [Z/H] = -2.3. Figure 1 in (36) shows three clusters with masses greater than  $10^6 M_{\odot}$  and metallicities below this limit, with a few clusters near the limit.

## Supplementary Text

### Comparison with the metal-poor globular cluster Hodge III

In Figure S2 we compare the EXT8 spectrum with a spectrum of the globular cluster Hodge III in the M31 satellite dwarf galaxy NGC 147. Hodge III has a low metallicity of  $[\text{Fe}/\text{H}] = -2.48$  with an rms dispersion of 0.154 dex from model fits to 25 spectral orders (18), and its spectrum was obtained with the same HIRES configuration as that of EXT8. Hodge III has a smaller velocity dispersion than EXT8 and the two spectra have therefore been broadened to the same resolution to allow direct comparison. While the spectrum of Hodge III is noisier than those of M15 and EXT8, Figure S2 shows that the spectral features are much weaker in the spectrum EXT8, consistent with its lower metallicity.

### Modeling the weaker Mg I lines

In Figure S3 we show the best-fitting models for the three weaker Mg I lines at 4571 Å, 4703 Å, and 5528 Å. The magnesium abundances derived from the modeling of these lines are consistent with the  $[\text{Mg}/\text{Fe}]$  ratio derived from the stronger Mg I *b* lines, but do not strongly constrain the  $[\text{Mg}/\text{Fe}]$  ratio for EXT8.

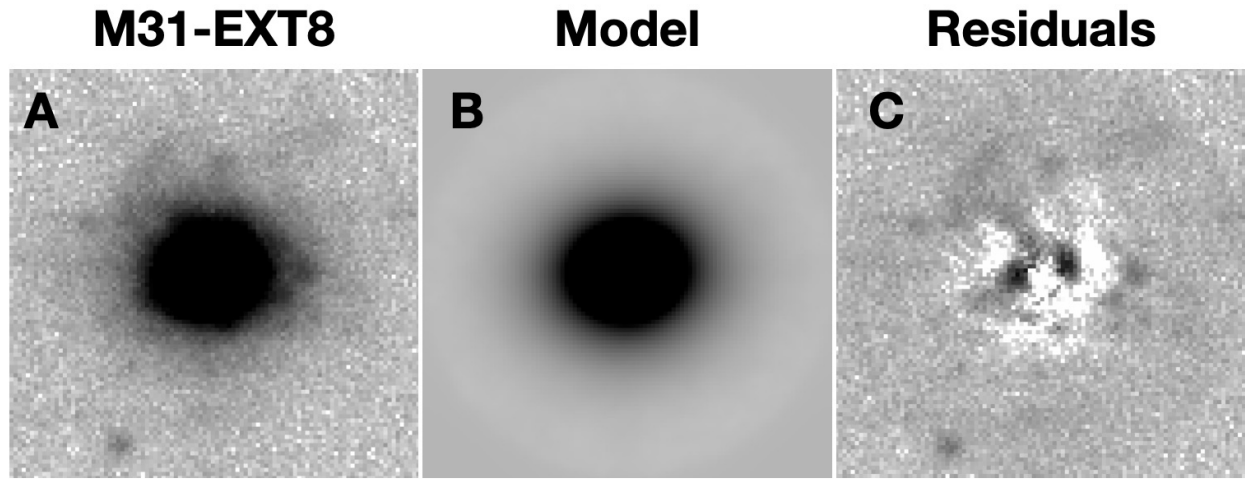

**Figure S1. King model fit to MegaCam image of EXT8.** Panel (A) shows one of the 100 s MegaCam exposures of EXT8, Panel (B) the best-fitting King model convolved with the point-spread function, and Panel (C) the residual difference between panels (A) and (B). Each panel measures  $100 \times 100$  pixels or about  $70 \times 70$  parsec at the distance of M31.

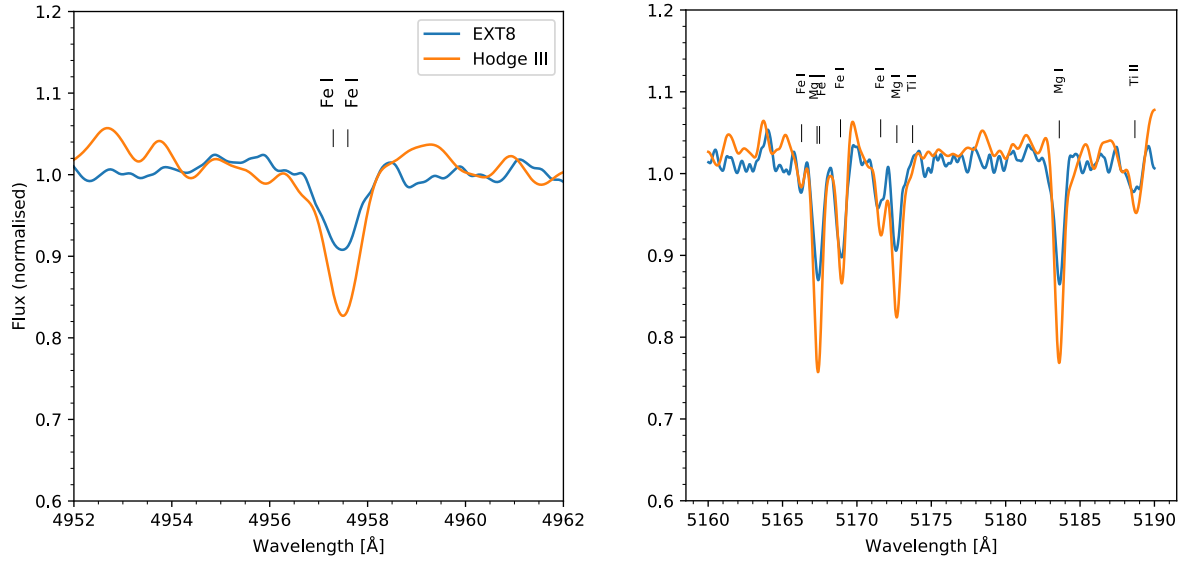

**Figure S2. Spectra of EXT8 and Hodge III.** Both spectra were obtained with HIRES and they have here been broadened to the same resolution to facilitate comparison.

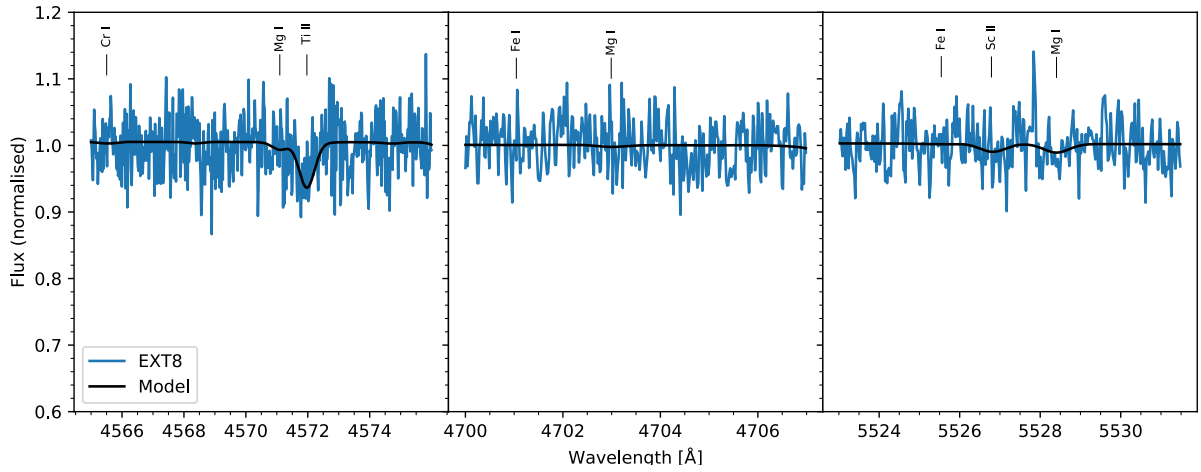

**Figure S3. Model-data comparison for the weaker Mg I lines.** The blue line shows the observed spectrum of EXT8 and the black line shows the model.

**Table S1. HRD bins used for analysis of the spectrum of EXT8.** The HRD bins are based on a MIST isochrone with  $[\text{Fe}/\text{H}] = -2.7$  and an age of 12.5 Gyr. The columns are:  $m$  = initial stellar mass,  $T_{\text{eff}}$  = effective temperature,  $\log g$  = logarithm of surface gravity,  $R$  = stellar radius,  $w$  = weight (number of stars),  $L_{500\text{nm}}$  is the fractional contribution to the luminosity at 500 nm, and  $\log V_t$  = logarithm of microturbulent velocity.

| $m [M_{\odot}]$ | $T_{\text{eff}} [\text{K}]$ | $\log g [\text{cm s}^{-2}]$ | $R [R_{\odot}]$ | $w$       | $L_{500\text{nm}}$ | $\log V_t [\text{km s}^{-1}]$ |
|-----------------|-----------------------------|-----------------------------|-----------------|-----------|--------------------|-------------------------------|
| 0.131           | 3922.4                      | 5.2756                      | 0.137           | 9571.870  | 0.0005             | -0.301                        |
| 0.149           | 4041.2                      | 5.2135                      | 0.157           | 8543.628  | 0.0007             | -0.301                        |
| 0.180           | 4137.5                      | 5.1485                      | 0.186           | 11924.318 | 0.0015             | -0.301                        |
| 0.220           | 4206.2                      | 5.0859                      | 0.222           | 11590.944 | 0.0023             | -0.301                        |
| 0.261           | 4244.7                      | 5.0421                      | 0.254           | 9483.719  | 0.0026             | -0.301                        |
| 0.293           | 4272.5                      | 5.0168                      | 0.277           | 6400.695  | 0.0021             | -0.301                        |
| 0.319           | 4305.1                      | 4.9999                      | 0.296           | 4723.770  | 0.0019             | -0.301                        |
| 0.365           | 4372.3                      | 4.9774                      | 0.325           | 6997.894  | 0.0037             | -0.301                        |
| 0.416           | 4493.5                      | 4.9289                      | 0.366           | 6445.750  | 0.0052             | -0.301                        |
| 0.455           | 4620.3                      | 4.8873                      | 0.402           | 4424.955  | 0.0051             | -0.301                        |
| 0.489           | 4766.8                      | 4.8490                      | 0.435           | 3411.779  | 0.0055             | -0.301                        |
| 0.523           | 4962.3                      | 4.8105                      | 0.471           | 3117.925  | 0.0075             | -0.301                        |
| 0.558           | 5195.2                      | 4.7718                      | 0.508           | 2702.336  | 0.0097             | -0.301                        |
| 0.591           | 5437.9                      | 4.7327                      | 0.547           | 2241.359  | 0.0118             | -0.301                        |
| 0.624           | 5698.4                      | 4.6867                      | 0.593           | 2015.284  | 0.0157             | -0.301                        |
| 0.655           | 5937.1                      | 4.6394                      | 0.641           | 1622.968  | 0.0179             | -0.301                        |
| 0.690           | 6181.5                      | 4.5972                      | 0.686           | 1698.809  | 0.0259             | -0.301                        |
| 0.721           | 6412.9                      | 4.5498                      | 0.737           | 1308.063  | 0.0273             | -0.301                        |
| 0.745           | 6622.9                      | 4.4964                      | 0.794           | 985.493   | 0.0278             | 0.000                         |
| 0.765           | 6802.5                      | 4.4365                      | 0.860           | 735.696   | 0.0278             | 0.000                         |
| 0.780           | 6944.6                      | 4.3693                      | 0.937           | 549.592   | 0.0273             | 0.000                         |
| 0.792           | 7045.4                      | 4.2944                      | 1.028           | 412.692   | 0.0266             | 0.000                         |
| 0.801           | 7098.6                      | 4.2113                      | 1.137           | 311.346   | 0.0256             | 0.000                         |
| 0.807           | 7081.4                      | 4.1215                      | 1.265           | 208.287   | 0.0211             | 0.000                         |
| 0.812           | 6992.1                      | 4.0234                      | 1.420           | 133.600   | 0.0161             | 0.000                         |
| 0.816           | 6687.9                      | 3.8288                      | 1.780           | 131.510   | 0.0203             | 0.024                         |
| 0.818           | 6352.3                      | 3.6146                      | 2.280           | 74.104    | 0.0147             | 0.052                         |
| 0.820           | 6090.4                      | 3.4061                      | 2.901           | 53.525    | 0.0141             | 0.078                         |
| 0.821           | 5858.5                      | 3.2004                      | 3.679           | 41.588    | 0.0146             | 0.103                         |
| 0.822           | 5639.0                      | 2.9950                      | 4.662           | 33.568    | 0.0157             | 0.125                         |
| 0.823           | 5462.1                      | 2.7844                      | 5.943           | 31.399    | 0.0203             | 0.148                         |
| 0.824           | 5360.5                      | 2.5688                      | 7.619           | 26.226    | 0.0253             | 0.169                         |
| 0.824           | 5266.4                      | 2.3528                      | 9.769           | 20.642    | 0.0300             | 0.190                         |
| 0.825           | 5169.5                      | 2.1348                      | 12.551          | 16.044    | 0.0348             | 0.210                         |
| 0.825           | 5069.1                      | 1.9150                      | 16.152          | 12.496    | 0.0402             | 0.229                         |
| 0.826           | 4965.2                      | 1.6957                      | 20.766          | 9.269     | 0.0436             | 0.248                         |

|       |         |        |        |        |        |       |
|-------|---------|--------|--------|--------|--------|-------|
| 0.826 | 4856.3  | 1.4711 | 26.850 | 6.722  | 0.0459 | 0.266 |
| 0.826 | 4801.4  | 1.3583 | 30.539 | 3.049  | 0.0249 | 0.274 |
| 0.826 | 4761.8  | 1.2738 | 33.610 | 2.942  | 0.0275 | 0.281 |
| 0.826 | 4707.5  | 1.1605 | 38.229 | 2.101  | 0.0233 | 0.289 |
| 0.826 | 4653.8  | 1.0466 | 43.496 | 1.850  | 0.0244 | 0.298 |
| 0.826 | 4602.0  | 0.9327 | 49.462 | 1.616  | 0.0251 | 0.301 |
| 0.826 | 4554.2  | 0.8201 | 56.127 | 1.426  | 0.0260 | 0.301 |
| 0.826 | 4538.0  | 0.7754 | 58.989 | 0.581  | 0.0113 | 0.301 |
| 0.826 | 4648.5  | 0.9646 | 47.442 | 0.008  | 0.0001 | 0.301 |
| 0.826 | 11180.6 | 3.7605 | 1.898  | 1.204  | 0.0012 | 0.033 |
| 0.826 | 11677.0 | 3.8836 | 1.647  | 0.078  | 0.0001 | 0.017 |
| 0.828 | 10975.5 | 3.7346 | 1.957  | 57.575 | 0.0610 | 0.037 |
| 0.829 | 9598.7  | 3.4128 | 2.835  | 24.443 | 0.0411 | 0.078 |
| 0.829 | 9375.5  | 3.3402 | 3.083  | 10.205 | 0.0192 | 0.086 |
| 0.830 | 8810.2  | 3.1215 | 3.966  | 9.542  | 0.0253 | 0.112 |
| 0.830 | 8266.4  | 2.9689 | 4.728  | 0.261  | 0.0008 | 0.128 |
| 0.830 | 7589.4  | 2.7776 | 5.892  | 1.413  | 0.0048 | 0.148 |
| 0.830 | 6958.1  | 2.5737 | 7.452  | 1.473  | 0.0053 | 0.169 |
| 0.830 | 6377.8  | 2.3695 | 9.426  | 1.097  | 0.0041 | 0.189 |
| 0.830 | 5846.5  | 2.1668 | 11.903 | 1.032  | 0.0040 | 0.207 |
| 0.830 | 5401.8  | 1.9446 | 15.373 | 0.984  | 0.0041 | 0.227 |
| 0.830 | 5145.2  | 1.7110 | 20.112 | 1.072  | 0.0059 | 0.246 |
| 0.830 | 4986.0  | 1.4925 | 25.853 | 1.106  | 0.0083 | 0.264 |
| 0.830 | 4855.7  | 1.2850 | 32.806 | 0.851  | 0.0086 | 0.280 |
| 0.830 | 4770.8  | 1.1433 | 38.601 | 0.391  | 0.0049 | 0.291 |

**Table S2. Average abundances for EXT8.** The last column,  $N$ , gives the number of individual measurements, listed in Tables S3-S9. For sodium we list the average of the two measurements of the  $D$  lines. For magnesium we list the value obtained from the Mg I  $b$  triplet.

| Element | Value  | Error | rms   | $N$ |
|---------|--------|-------|-------|-----|
| [Fe/H]  | -2.908 | 0.039 | 0.175 | 21  |
| [Na/Fe] | +0.229 | 0.073 | -     | 1   |
| [Mg/Fe] | -0.352 | 0.050 | -     | 1   |
| [Si/Fe] | +0.648 | 0.313 | -     | 1   |
| [K/Fe]  | +0.668 | 0.149 | -     | 1   |
| [Ca/Fe] | +0.345 | 0.070 | 0.172 | 7   |
| [Ti/Fe] | +0.192 | 0.058 | 0.154 | 8   |

**Table S3. Iron abundances.** For each echelle order, the wavelength range, the measured [Fe/H], and the associated uncertainty are listed.

| Wavelength range | [Fe/H] | Uncertainty |
|------------------|--------|-------------|
| 4370.4-4437.9    | −2.512 | 0.053       |
| 4424.9-4493.4    | −3.065 | 0.068       |
| 4480.9-4550.4    | −2.793 | 0.062       |
| 4538.2-4608.8    | −2.800 | 0.073       |
| 4597.1-4668.7    | −3.133 | 0.130       |
| 4657.5-4730.2    | −2.975 | 0.265       |
| 4719.5-4793.4    | −3.088 | 0.229       |
| 4783.2-4858.3    | −2.517 | 0.246       |
| 4848.6-4924.9    | −3.097 | 0.051       |
| 4915.9-4973.2    | −3.031 | 0.052       |
| 5064.3-5136.3    | −2.911 | 0.051       |
| 5129.4-5210.8    | −3.026 | 0.036       |
| 5204.7-5287.5    | −2.785 | 0.036       |
| 5282.3-5366.5    | −3.043 | 0.047       |
| 5362.3-5447.9    | −2.966 | 0.041       |
| 5444.7-5531.8    | −2.753 | 0.043       |
| 5529.7-5618.3    | −3.190 | 0.089       |
| 5707.9-5799.7    | −2.906 | 0.410       |
| 5801.3-5894.8    | −2.572 | 0.331       |
| 5997.8-6094.8    | −2.382 | 0.108       |
| 6101.2-6199.9    | −3.053 | 0.086       |

**Table S4. Sodium abundances for each wavelength range.** The Na *D* lines appear in two echelle orders, and are thus listed twice in the table.

| Wavelength range               | [Na/Fe] | Uncertainty        |
|--------------------------------|---------|--------------------|
| 5677.0-5695.0                  | +0.259  | +0.324 / $-\infty$ |
| 5882.0-5899.7 (Na I <i>D</i> ) | +0.259  | 0.088              |
| 5893.1-5902.0 (Na I <i>D</i> ) | +0.161  | 0.134              |

**Table S5. Magnesium abundance measurements.** The wavelength range at 5523-5531.5 Å appears in two echelle orders.

| Wavelength range               | [Mg/Fe] | Uncertainty        |
|--------------------------------|---------|--------------------|
| 4565.0-4576.0                  | -0.155  | 0.422              |
| 4700.0-4707.0                  | -0.957  | +0.647 / $-\infty$ |
| 5160.0-5190.0 (Mg I <i>b</i> ) | -0.352  | 0.050              |
| 5523.0-5531.5                  | -0.296  | 0.319              |
| 5524.8-5531.5                  | -0.433  | 0.393              |

**Table S6. Silicon abundance.**

| <b>Wavelength range</b> | <b>[Si/Fe]</b> | <b>Uncertainty</b> |
|-------------------------|----------------|--------------------|
| 7400.0-7427.0           | +0.648         | 0.313              |

**Table S7. Potassium abundance.**

| <b>Wavelength range</b> | <b>[K/Fe]</b> | <b>Uncertainty</b> |
|-------------------------|---------------|--------------------|
| 7691.0-7706.0           | +0.668        | 0.149              |

**Table S8. Calcium abundance measurements.**

| <b>Wavelength range</b> | <b>[Ca/Fe]</b> | <b>Uncertainty</b> |
|-------------------------|----------------|--------------------|
| 4222.0-4232.0           | 0.622          | 0.121              |
| 4280.0-4320.0           | 0.238          | 0.105              |
| 4420.0-4460.0           | 0.441          | 0.085              |
| 4575.0-4591.0           | 0.576          | 0.165              |
| 5259.0-5268.0           | 0.686          | 0.143              |
| 5580.0-5610.0           | 0.232          | 0.111              |
| 6100.0-6175.0           | 0.203          | 0.060              |

**Table S9. Titanium abundance measurements.**

| <b>Wavelength range</b> | <b>[Ti/Fe]</b> | <b>Uncertainty</b> |
|-------------------------|----------------|--------------------|
| 4292.0-4320.0           | +0.433         | 0.092              |
| 4440.0-4474.0           | +0.091         | 0.101              |
| 4533.3-4574.0           | +0.123         | 0.076              |
| 4587.0-4593.0           | +0.054         | 0.208              |
| 4652.6-4715.0           | −0.282         | 0.810              |
| 4750.0-4785.0           | +0.203         | 0.256              |
| 4785.0-4850.0           | −0.189         | 0.459              |
| 5152.0-5160.0           | −0.013         | 0.449              |

**Table S10. Results of King profile model fits.** For each of the three MegaCam images and three different fitting radii ( $R_{fit}=25, 50$ , and  $100$  pixels), the quantities are: FWHM (Full Width at Half Maximum) of the King profile, the minor/major axis ratio, the concentration parameter ( $R_{tidal}/R_{core}$  for core radius  $R_{core}$ ), tidal radius  $R_{tidal}$ , the semi-major axis of the elliptical profile containing half of the cluster light  $R_{eff}(\text{ell})$ , and the radius of a circular aperture containing half of the cluster light  $R_{eff}(\text{circ})$ .

| Dataset                                | FWHM<br>[pixels] | Minor/Major | Concentration | $R_{tidal}$<br>[pixels] | $R_{eff}(\text{ell})$<br>[pixels] | $R_{eff}(\text{circ})$<br>[pixels] |
|----------------------------------------|------------------|-------------|---------------|-------------------------|-----------------------------------|------------------------------------|
| <b><math>R_{fit}=25</math> pixels</b>  |                  |             |               |                         |                                   |                                    |
| 2011389                                | 2.77             | 0.81        | 28.04         | 40                      | 3.94                              | 3.57                               |
| 2011390                                | 2.75             | 0.81        | 29.39         | 41                      | 4.00                              | 3.62                               |
| 2011391                                | 2.70             | 0.81        | 30.08         | 42                      | 3.97                              | 3.59                               |
| Mean                                   |                  |             |               |                         | 3.97                              | 3.59                               |
| <b><math>R_{fit}=50</math> pixels</b>  |                  |             |               |                         |                                   |                                    |
| 2011389                                | 2.47             | 0.81        | 44.41         | 56                      | 4.35                              | 3.94                               |
| 2011390                                | 2.41             | 0.81        | 47.66         | 59                      | 4.39                              | 3.97                               |
| 2011391                                | 2.34             | 0.82        | 49.27         | 59                      | 4.33                              | 3.94                               |
| Mean                                   |                  |             |               |                         | 4.36                              | 3.95                               |
| <b><math>R_{fit}=100</math> pixels</b> |                  |             |               |                         |                                   |                                    |
| 2011389                                | 2.24             | 0.82        | 62.01         | 71                      | 4.61                              | 4.20                               |
| 2011390                                | 2.17             | 0.81        | 71.21         | 78                      | 4.77                              | 4.32                               |
| 2011391                                | 2.12             | 0.82        | 71.22         | 76                      | 4.66                              | 4.24                               |
| Mean                                   |                  |             |               |                         | 4.68                              | 4.25                               |
